# Supplementary material for: Generative Panoramic Image Stitching
Source: arXiv:2507.07133 source file (2025-07-08)

proposed

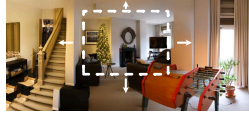

RealFill

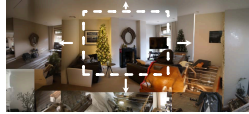

AutoStitch

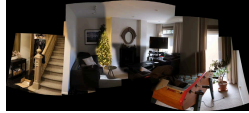

input

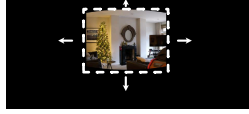

ref. images

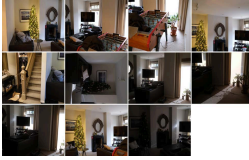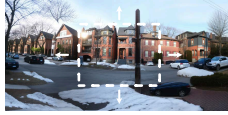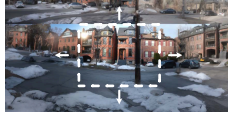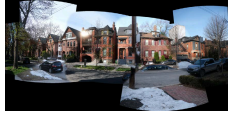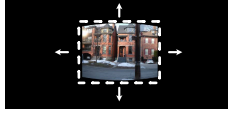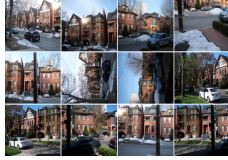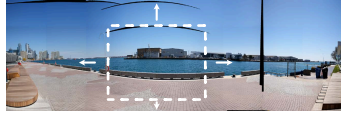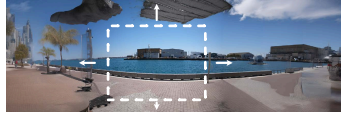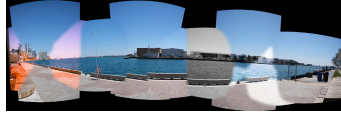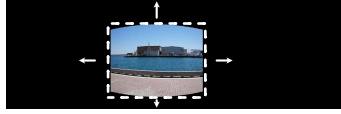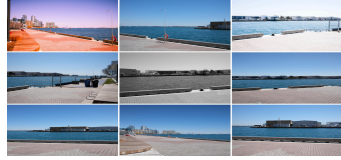

proposed

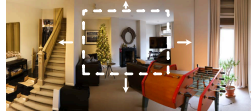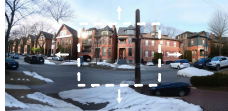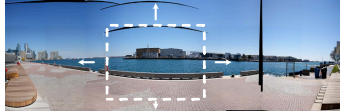

RealFill

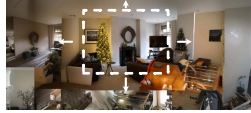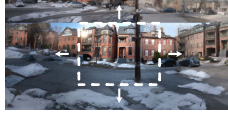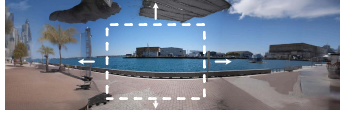

AutoStitch

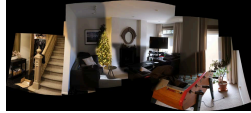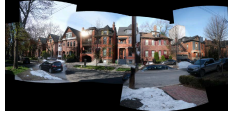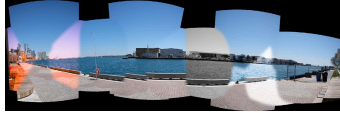

input

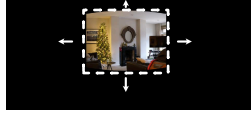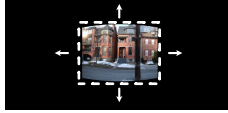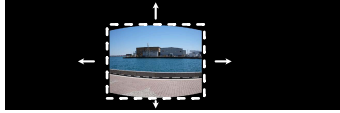

ref. images

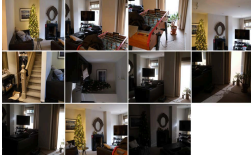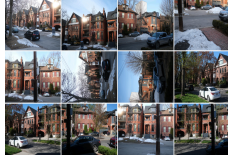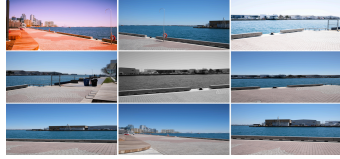

Supplement: Supplementary file 1 [file results-supp-casual.pdf]
